# Supplementary material for: Text and Patterns: For Effective Chain of Thought, It Takes Two to Tango
Source: arXiv:2209.07686 source file (2022-10-13)
Supplement: Supplementary file 1 [file counterfactual.tex]

\section{Counterfactual Inference}
\label{sec:counterfactual}

\newcommand{\nd}[2]{\node[circle,minimum size=18pt, align=center,yshift=6cm,xshift=-4cm] (S) {$S$}}

\newcommand{\symb}{$S$\xspace}
\newcommand{\pat}{$P$\xspace}
\newcommand{\txt}{$T$\xspace}
\newcommand{\out}{$y$\xspace}
\newcommand{\conf}{$C$\xspace}

We utilize multiple datasets in this work, and have task specific definitions of symbols \symb, patterns \pat, and text \txt.
However, the main design of our experiments is simple and consistent across all dataset.
In this section, we factor out our methodology in a causal graph shown in \Cref{fig:cfgraph}.

Note that there are three different counterfactual graphs that are related to our work: \begin{inparaenum} \item training data generation, \item prompt creation, \item model mechanism \end{inparaenum}
\Cref{fig:cfgraph} only captures one of them: prompt creation.

\begin{figure}[!ht]
  \centering
  \tikz{ %
    \node[circle, draw=black!80, minimum size=32pt, align=center,yshift=6cm,xshift=-2cm] (S) {\symb} ;
    \node[circle, draw=black!80, minimum size=32pt, align=center,yshift=4cm,xshift=-4cm,] (PAT) {\pat} ;
    \node[circle, draw=black!80, minimum size=32pt, align=center,yshift=4cm,xshift=-6cm,] (T) {\txt} ;
    \node[circle, draw=black!80, minimum size=32pt, align=center,yshift=0cm,xshift=-4cm,] (p) {\pcot} ;
    \node[circle, draw=black!80, minimum size=32pt, align=center,yshift=-3cm,xshift=-4cm,] (y) {\out} ;
    \node[circle, draw=black!80, minimum size=32pt, align=center,yshift=8cm,xshift=-6cm,] (conf) {\conf} ;
    \edge {S} {PAT} ; %
    \edge {S} {PAT} ; %
    \edge {T} {p} ; %
    \path (S) edge [out = -40, in = 45,->] (p) ;
    \edge {PAT} {p} ; %
    \edge[dashed] {conf} {T} ; %
    \edge[dashed] {conf} {PAT} ; %
    \edge[dashed] {conf} {S} ; %
    \edge {p} {y} ;
  }
 \caption{Counterfactual graph for our work: symbols \symb, patterns \pat, text \txt are the key components of our work. The outcome is binary \out (accuracy). We make a simplifying assumption that these are identifiable. \symb and \text may be confounded by an unidentifiable \conf, and this is a limitation of our work.}
 \label{fig:cfgraph}
\end{figure}

\niparagraph{Average treatment effect.}
Let \cfprompt{z} be a counterfactual prompt obtained by changing all except one of \symb, \pat, and \txt.
We estimate the average treatment effect (ATE) of such counterfactual prompt as:

\begin{align*}
    ATE &= \mathbb{E}_D[y(p) - y(C_z(p))]
\end{align*}

\noindent{}; where the expectation is calculated over the training data $D$.
For all our setups, ATE translates to the difference in accuracy for the original and counterfactual prompt.
Detailed experimental results are presented in \Cref{sec:mcnemar}.
