# Supplementary material for: Text and Patterns: For Effective Chain of Thought, It Takes Two to Tango
Source: arXiv:2209.07686 source file (2022-10-13)
Supplement: Supplementary file 2 [file notation.tex]

\section{Introduction and Glossary}
\label{sec:notation}
We explore how symbiosis of text and pattern leads to effective chain of thought prompting.
Our methodology focuses on two fronts:
\begin{enumerate}
    \item \niparagraph{Counterfactual prompts:} where the original \pcot are modified to either change symbols, patterns, or text.
    \item \niparagraph{Attention analysis:} where we look at the attention scores over the token to compare inference patterns when running inference with stream prompts vs. symbolic prompts.
\end{enumerate}

In this Appendix, we present additional results and methodology details that were omitted from the main draft for clarity.

\niparagraph{Glossary.} 
Throughout the main paper, we have experimented with a number of prompts.
For quick reference, all the counterfactual prompts are listed in \Cref{tab:all_counterfactual_thoughts} for \gsm. 
\begin{table}[!ht]
\small
\begin{tabular}{p{3cm}p{4cm}p{6cm}}
\toprule
\textbf{Prompt} & \textbf{Definition} & \textbf{Sample Thought} \\
\toprule
\direct  &  No thought is used. This is the baseline few-shot setup. & ---  \\ \midrule
\pcot &  Identical thoughts as \citet{wei2022chain} are used. & Shawn started with 5 toys. If he got 2 toys each from his mom and dad, then that is 4 more toys. 5 + 4 = 9.\\\toprule
\multicolumn{3}{c}{$\LHD\,$\bm{\symbhl{Symbols}}$\,\RHD$}\\\toprule
\psymbabs & All the symbols are replaced with abstract placeholders. & Shawn started with \symbhl{\bm{$\alpha$}} toys. If he got \symbhl{\bm{$\beta$}} toys each from his mom and dad, then that is \symbhl{\bm{$\lambda$}} more toys. \symbhl{\bm{$\alpha$}} + \symbhl{\bm{$\lambda$}} = \symbhl{\bm{$\pi$}}. \\  \midrule
\psymbood  & Symbols are replaced with out-of-distribution values. &  Shawn started with \symbhl{5.5} toys. If he got \symbhl{2.5} toys each from his mom and dad, then that is 5 more toys. \symbhl{5.5} + \symbhl{5} = \symbhl{10.5}. \\  \midrule
\multicolumn{3}{c}{$\LHD\,$\bm{\pathl{Patterns}}$\,\RHD$}\\\toprule
\pwrongpat & Patterns are changed to reflect incorrect final answer. & Shawn started with 5 toys. If he got 2 toys each from his mom and dad, then that is 4 more toys. 5 \pathl{+} 4 \pathl{=} 7. \\  \midrule
\pnopat &  Patterns are removed from the thought. & Shawn started with 5 toys. If he got 2 toys each from his mom and dad, then that is 4 more toys.\\  \midrule
\ponlypat & Only pattern is retained in thoughts. &  5 \pathl{+} (2 \pathl{*} 2) \pathl{=} 9. \\  \midrule
\multicolumn{3}{c}{$\LHD\,$\textbf{Text}$\,\RHD$}\\\toprule
\ptextdiffentities  & Replaced with different entities of the same type (e.g. Shawn $\mapsto$ Teddy, Toys $\mapsto$ Cookies). & Teddy started with 5 cookies. If he got 2 cookies each from his Jenna and Rehan, then that is 4 more cookies. 5 + 4 = 9.\\  \midrule
\ptextrand &  Random thought from a different example is used.& Capacity of one bus is 198 passengers / 9 buses = 22 passengers in one bus. Thus, 5 buses can fit 22 * 5 = 110 passengers.    \\  \midrule
\ptextyodathought  & Only the thought is changed to be in YodaSpeak~\citep{yodaspeech}. & With 5 toys, Shawn started. 2 toys each from his mom and dad, if he got, then that is 4 more toys. 5 + 4 = 9.     \\  \midrule
\ptextintershuf &   Tokens within each sentence of a thought are shuffled.    & dad, he got 5 toys. then started mom 2 each is more that from If his and toys. toys 4 with Shawn 5 + 4 = 9.     \\  \midrule
\ptextintrashuf  &  Tokens across sentences within a thought are shuffled.      & with Shawn toys 5 started. dad, from more 2 his toys then is toys he mom got that each 4 and If. 5 + 4 = 9. \\ \bottomrule
\end{tabular}%
\caption{The summary of the counterfactual prompts used in the main text.
The question is ``\hltext{Shawn has five toys. For Christmas, he got two toys each from his mom and dad. How many toys does he have now?}''.
Unless otherwise specified, different counterfactual prompts modify different parts of both thought and questions.}
\label{tab:all_counterfactual_thoughts}
\end{table}
